# Supplementary material for: MetaPred: Meta-Learning for Clinical Risk Prediction with Limited Patient Electronic Health Records
Source: arXiv:1905.03218 source file (2019-05-08)
Supplement: Supplementary file 1 [file 8-appendix.tex]

\appendix
\section*{Appendix}
\subsection*{A\quad Additional Details on the Dataset}

Table~\ref{tab:icd9} summarizes the ICD-9 codes for a set of cognition related disorders we identified within the OHSU dataset. %An underdiagnosis probably occur when doctors recognize one specific disease from others, which leads to a fairly challenging problem for disease diagnosis.

\begin{table}[t]
  \caption{Diagnosis codes of related diseases that set as cases or controls in disease diagnosis.}
  \vspace{-0.2cm}
  \label{tab:icd9}
  \begin{tabular}{ll}
  \toprule
    Disease  &ICD-9 Codes\\
    \midrule
    Mild Cognitive Impairment     &331.83, 331.89, 331.9 \\
    Alzheimer's Disease           &331.0, 331.2, 331.6, 331.7 \\
    Parkinson's Disease           &332.*	\\
    Dementia                      &290.*, 291.*, 294.*, 331.82 \\
    Amnesia                       &780.93   \\
    Huntington's Disease          &333.4\\
    Mechanical Obstructions   &331.3, 331.4, 331.5\\
    Frontotemporal Dementia   &331.1, 331.11, 331.19\\
    \bottomrule
\end{tabular}
\begin{tablenotes}
    \small
    \item $^*$ means that all the codes in this diagnosis group are included.
  \end{tablenotes}
\end{table}

% \section{B}
